# Supplementary material for: MS-UNIQUE: Multi-model and Sharpness-weighted Unsupervised Image Quality Estimation
Source: arXiv:1811.08947 ancillary file (2018-11-21)
Supplement: Supplementary file 1 [file Temel2017_EI_Slides.pdf]

***MS-UNIQUE:  
Multi-model and Sharpness-weighted  
Unsupervised Image Quality Estimation***

M. Prabhushankar, D. Temel, and G. AlRegib

Center for Signal and Information Processing  
School of Electrical and Computer Engineering  
Georgia Institute of Technology  
Atlanta, GA

## I. Introduction

## II. Literature Review

## III. UNIQUE: Unsupervised Image Quality Estimation

- *Overview of UNIQUE*
- *Unsupervised Learning Mechanism*
- *Preprocessing*
- *Visualization*

## IV. MS-UNIQUE: Multi-model and Sharpness-weighted UNIQUE

- *Multi-model*
- *Sharpness-weighted Multi-model*
- *Visualization*

## V. Validation

## VI. Conclusion

# I. Introduction

## Image Quality Assessment : Why?

| Application                                                                       | Average daily shared photos <sup>[1]</sup> |
|-----------------------------------------------------------------------------------|--------------------------------------------|
| 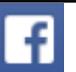 | 390 Million                                |
| 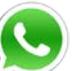 | 700 Million                                |
| 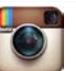 | 70 Million                                 |
| 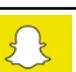 | 760 Million                                |

YouTube

NETFLIX

HBO

### Remote Assistance

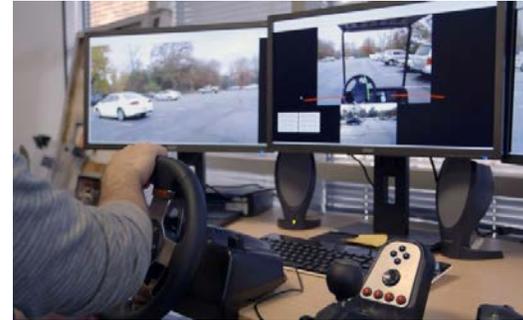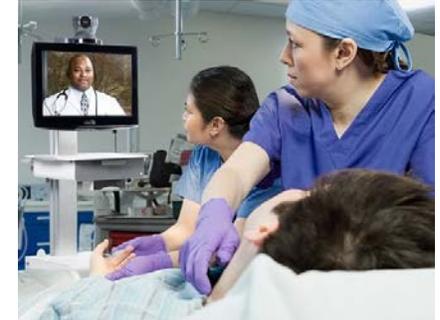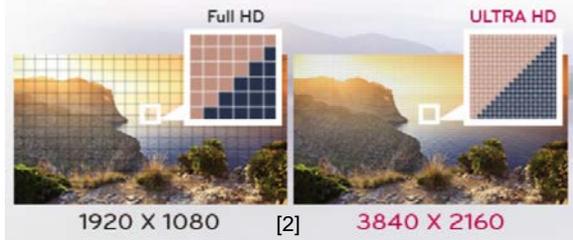

### Smart Capturing

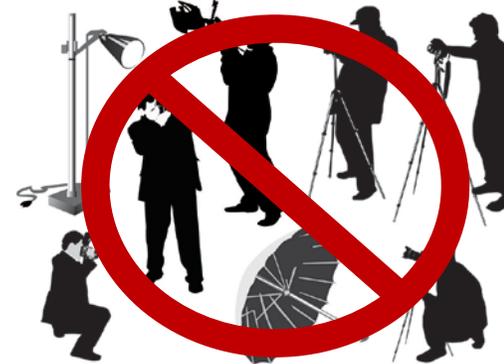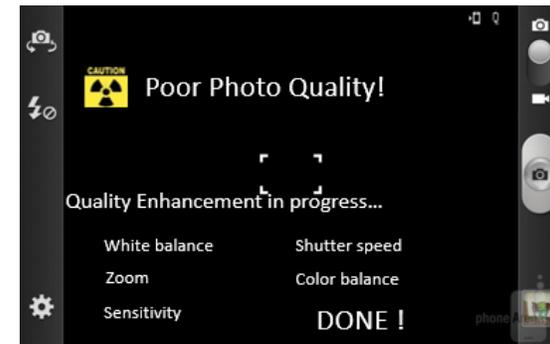

[3] 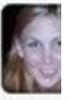 Mike Krieger @mikeyk

@sheepchase @\_kyliejane the changes **don't** **increase** the amount of **data** transferred--we put a lot of research into the **right balance**

Mike Krieger @mikeyk · Jul 6  
@aDam\_Nerd we did a lot of work on **image optimization** so **network bandwidth** should **not be affected**

[1] Adweek, <http://www.adweek.com/socialtimes/how-many-photos-are-uploaded-to-snapchat-every-second/621488>, Jun 2015  
 [2] LG, "Ultra Clarity, Ultra Scale," [http://www.lg.com/levant\\_en/Mini-page-ultra/index](http://www.lg.com/levant_en/Mini-page-ultra/index)  
 [3] PetPixel, <http://petapixel.com/2015/07/08/instagram-resolution-increase-heres-how-it-affects-image-quality-and-file-size/>, July 8, 2015

# I. Introduction

## Image Quality Assessment : In Practice

Test setup

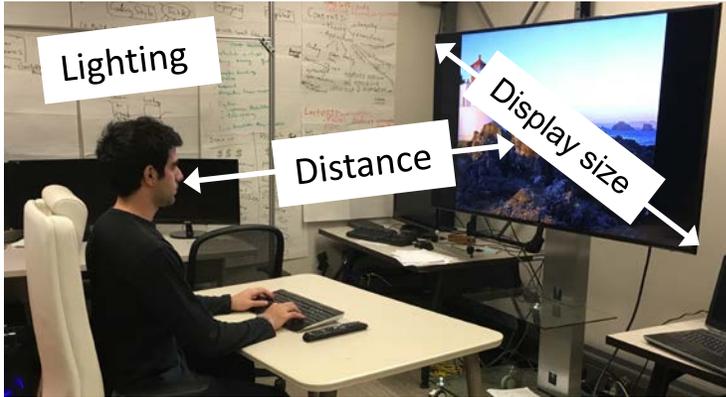

Reference images [1]

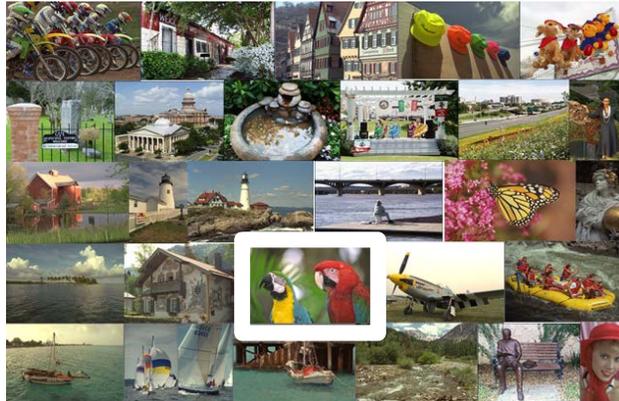

Distorted images [1]

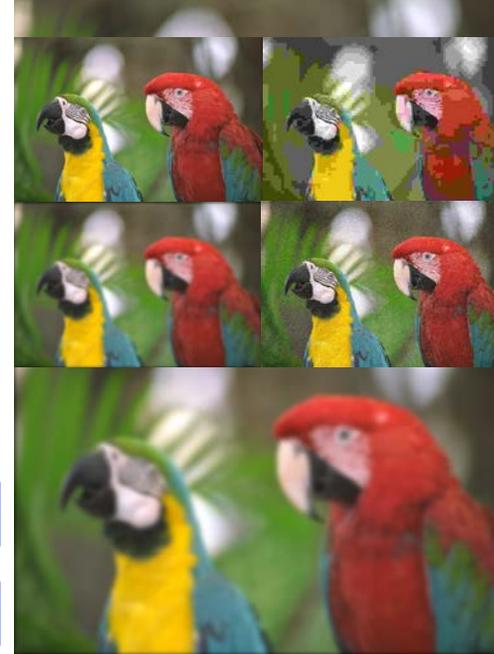

Subjective Scores

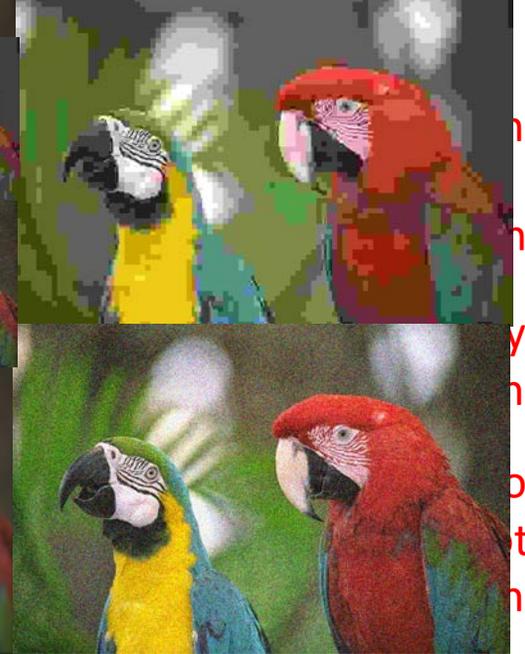

5 → Very Good no perceived distortion

Mean opinion scores

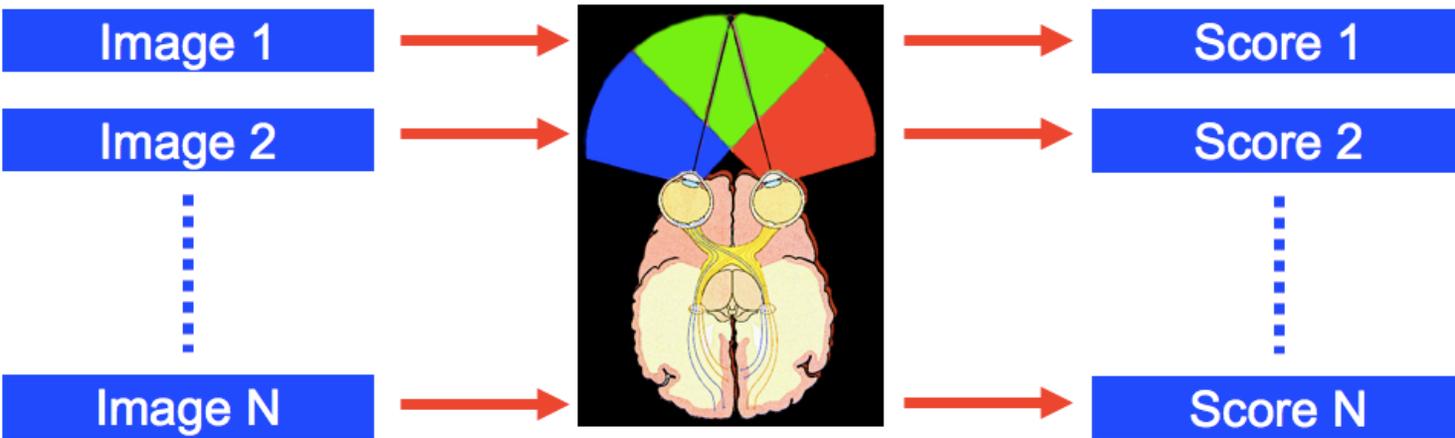

[1] Sheikh, H.R., Wang, Z., Cormack, L. and Bovik, A.C., "LIVE Image Quality Assessment Database Release 2", <http://live.ece.utexas.edu/research/quality>.

## I. Introduction

## II. Literature Review

## III. UNIQUE: Unsupervised Image Quality Estimation

- *Overview of UNIQUE*
- *Unsupervised Learning Mechanism*
- *Preprocessing*
- *Visualization*

## IV. MS-UNIQUE: Multi-model and Sharpness-weighted UNIQUE

- *Multi-model*
- *Sharpness-weighted Multi-model*
- *Visualization*

## V. Validation

## VI. Conclusion

# II. Literature Review

## Data-driven Image Quality Estimators

| YEAR                                        |                                          | 2011 |        | 2012   |         |       | 2013  |     |       | 2014 |     |      |                                            | 2015      |    |                               |       | 2016 |         |        |           |
|---------------------------------------------|------------------------------------------|------|--------|--------|---------|-------|-------|-----|-------|------|-----|------|--------------------------------------------|-----------|----|-------------------------------|-------|------|---------|--------|-----------|
| QUALITY ESTIMATORS                          |                                          | LBIQ | DIVINE | CORNIA | BRISQUE | MLIQM | CB/SF | QAC | SPARQ | Tang | QAF | Kang | Q <sub>area</sub><br>Q <sub>exponent</sub> | IQA-CNN++ | Li | S <sup>2</sup> F <sup>2</sup> | DLIQA | Gao  | CNN-SVR | UNIQUE | MS-UNIQUE |
| Visual system                               |                                          |      | ■      |        | ■       | ■     |       | ■   | ■     |      |     |      |                                            |           | ■  | ■                             | ■     | ■    |         | ■      | ■         |
| Color                                       |                                          |      |        |        |         | ■     |       |     |       |      |     |      |                                            |           |    |                               |       |      |         |        |           |
| Do not require                              | Distortion specific data in the training |      |        |        |         |       |       |     | ■     |      |     |      | ■                                          |           |    |                               |       |      |         |        |           |
|                                             | Labels in the training                   |      |        |        |         |       |       | ■   | ■     |      |     |      | ■                                          |           |    |                               |       |      |         |        |           |
|                                             | Handcrafting features                    |      |        | ■      |         |       | ■     |     |       |      |     | ■    |                                            | ■         |    |                               |       |      | ■       | ■      | ■         |
| Multiple layers/models without handcrafting |                                          |      |        |        |         |       |       |     |       |      |     | ■    |                                            | ■         | ■  |                               |       |      | ■       |        | ■         |

## I. Introduction

## II. Literature Review

## III. UNIQUE: Unsupervised Image Quality Estimation

- *Overview of UNIQUE*
- *Unsupervised Learning Mechanism*
- *Preprocessing*
- *Visualization*

## IV. MS-UNIQUE: Multi-model and Sharpness-weighted UNIQUE

- *Multi-model*
- *Sharpness-weighted Multi-model*

## V. Validation

## VI. Conclusion

### III. UNIQUE: Unsupervised Image Quality Estimation

Overview of UNIQUE

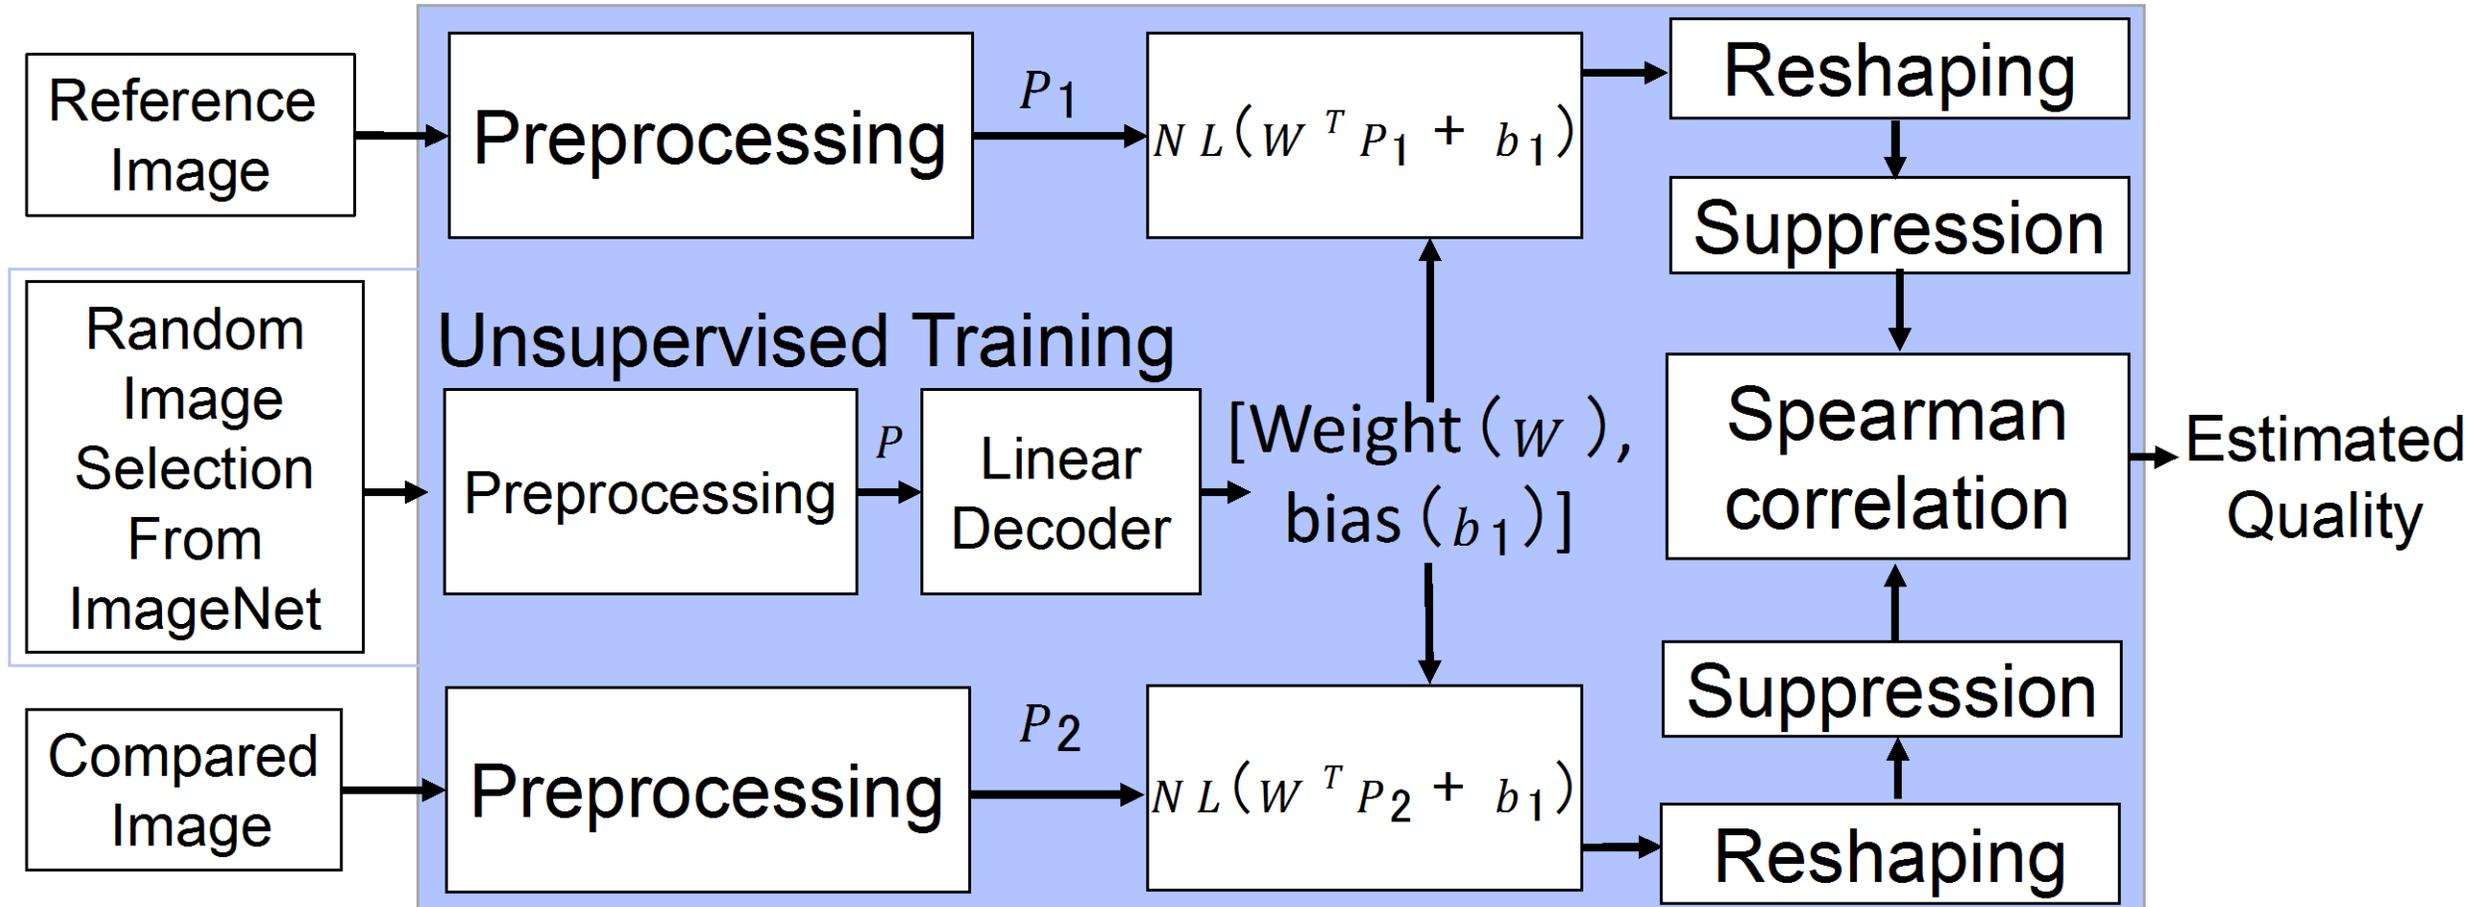

D. Temel, M. Prabhushankar, and G. AlRegib, "UNIQUE: Unsupervised Image Quality Estimation," the *IEEE Signal Processing Letters*, vol.23, no.10, pp.1414-1418.

# III. UNIQUE: Unsupervised Image Quality Estimation

Preprocessing

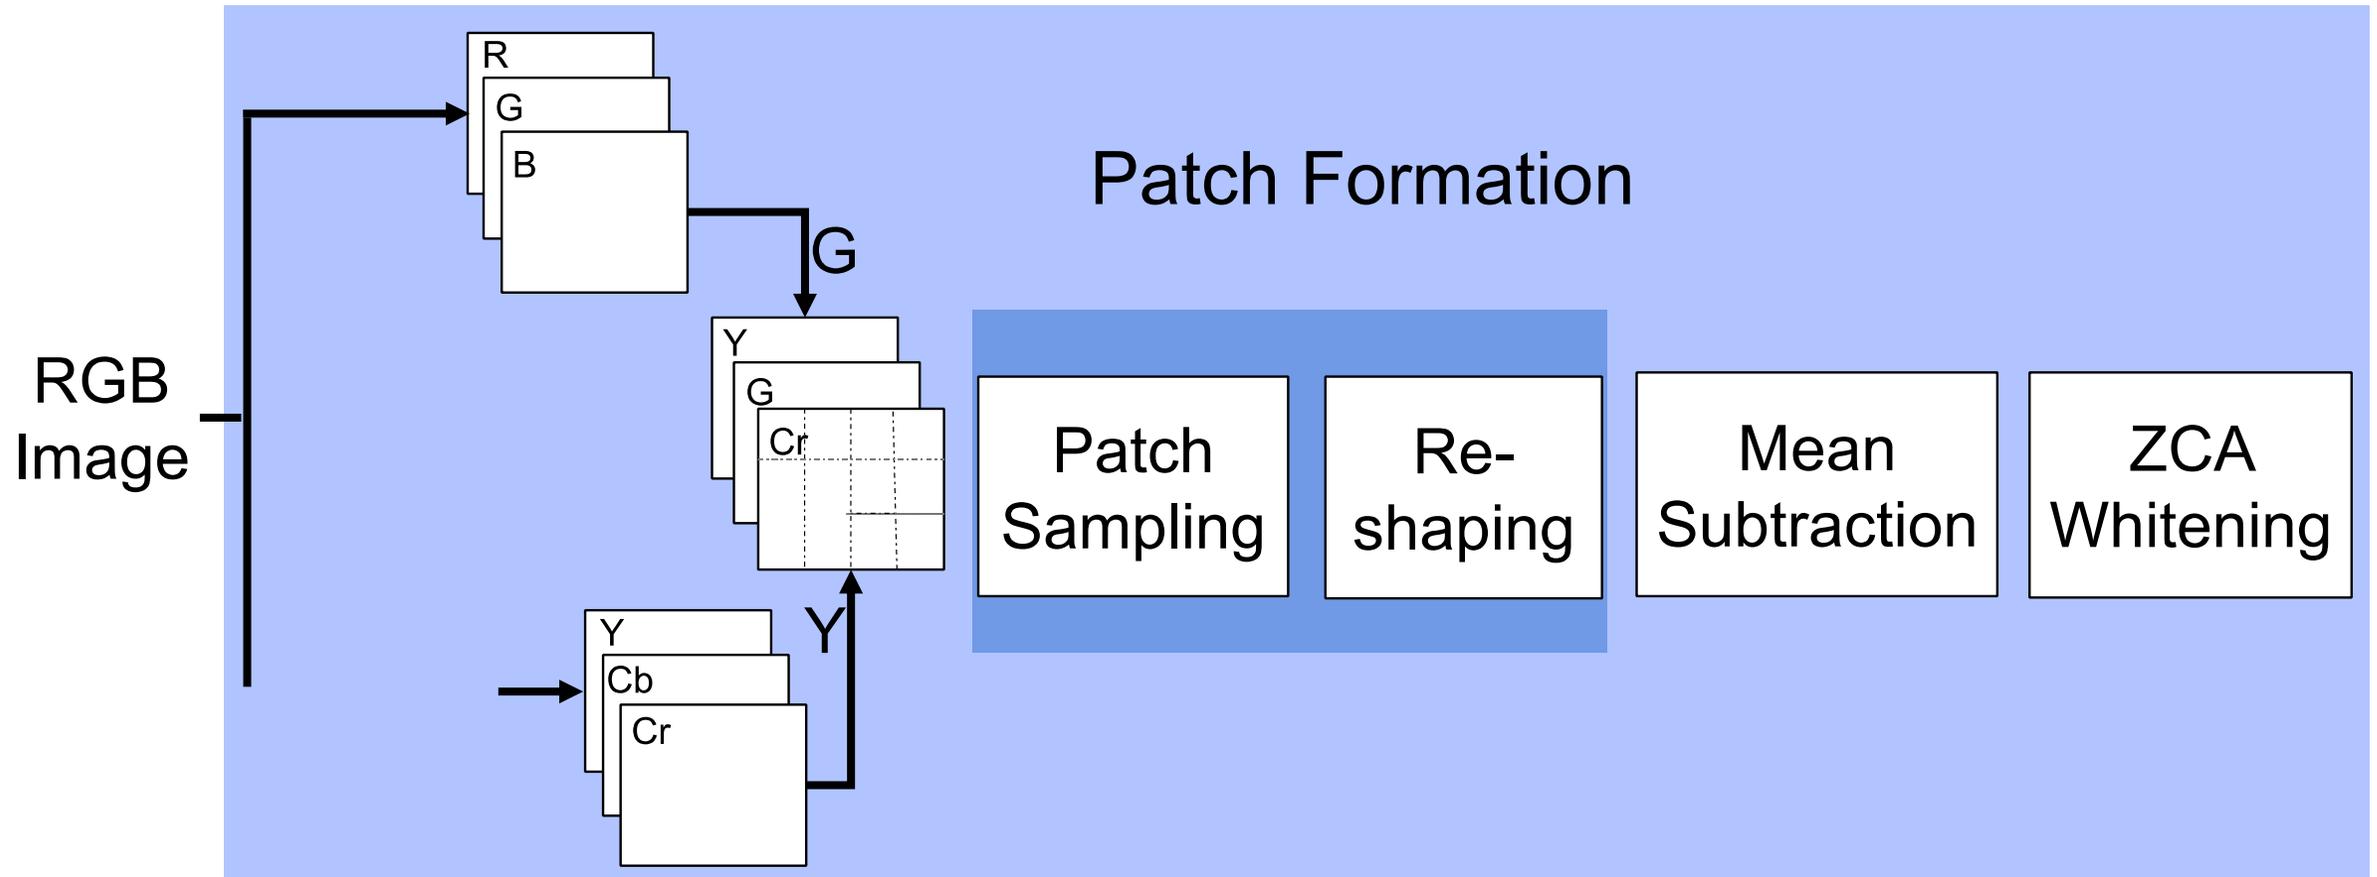

D. Temel, M. Prabhushankar, and G. AlRegib, "UNIQUE: Unsupervised Image Quality Estimation," the *IEEE Signal Processing Letters*, vol.23, no.10, pp.1414-1418.

### III. UNIQUE: Unsupervised Image Quality Estimation

Unsupervised Learning Mechanism

$$J(W_1, W_2, b_1, b_2) = \|(W_2^T s + b_2) - P\|_2^2 + \beta \|s\|_1 + \lambda \|W\|_2^2,$$

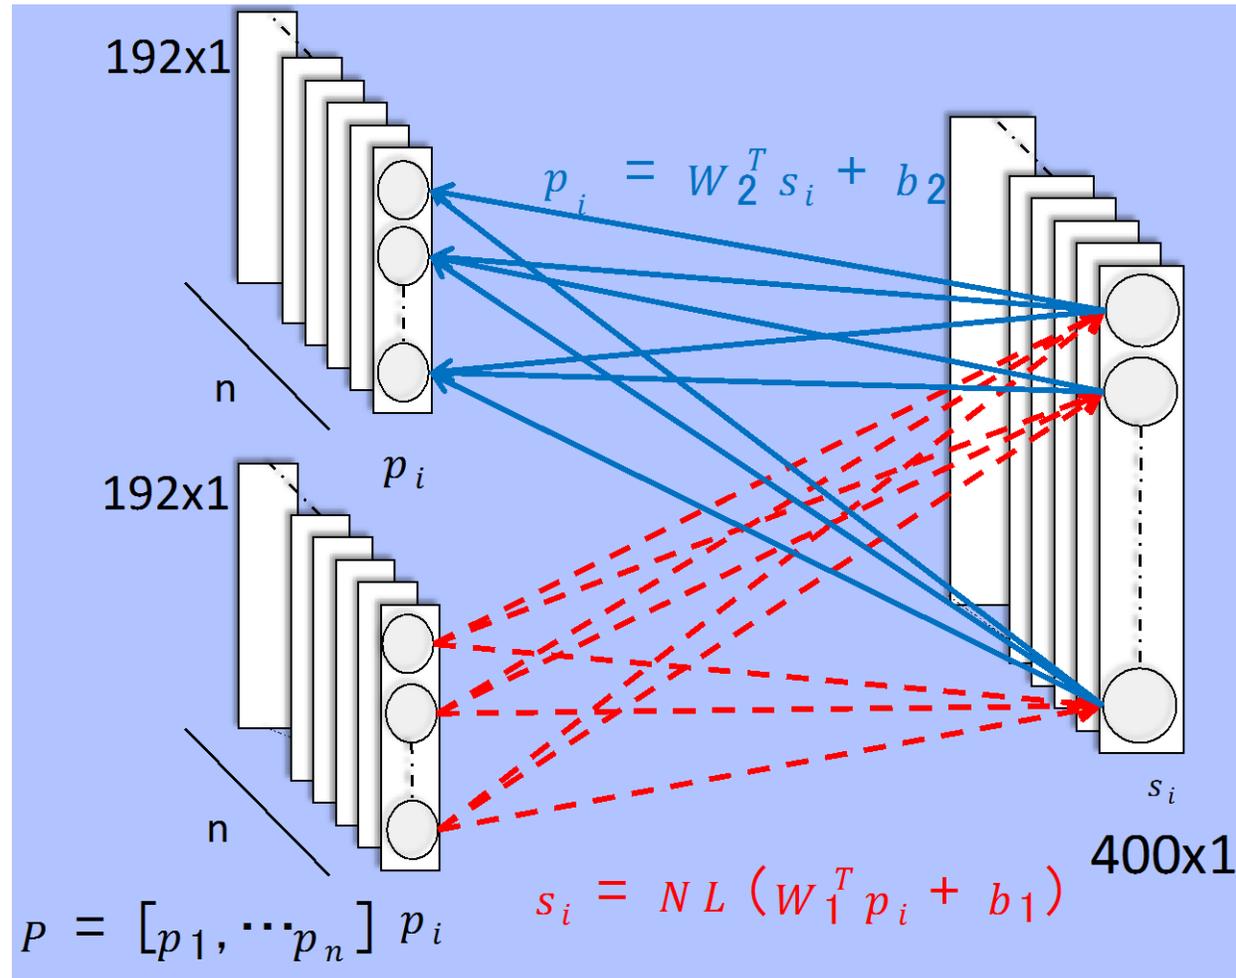

### III. UNIQUE: Unsupervised Image Quality Estimation

Visualization

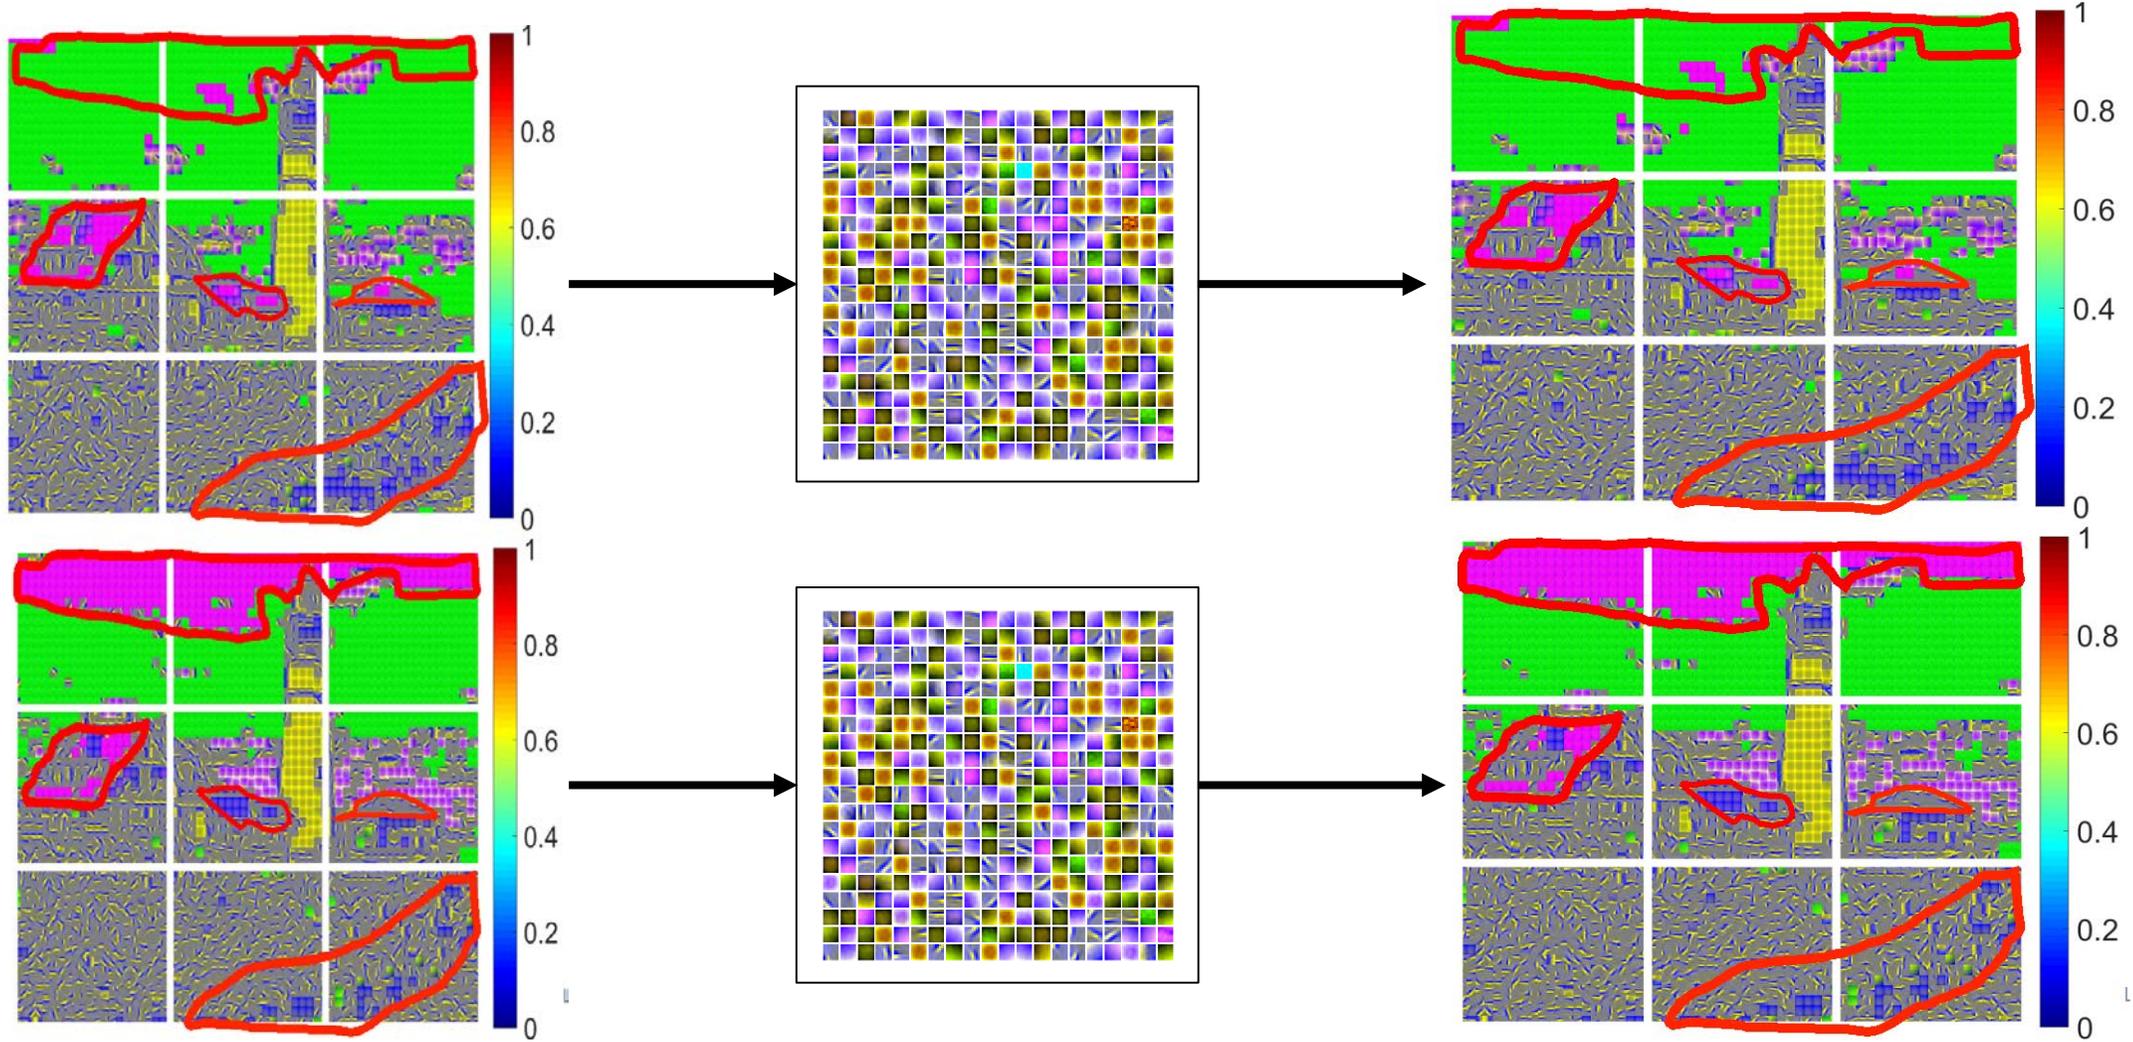

## I. Introduction

## II. Literature Review

## III. UNIQUE: Unsupervised Image Quality Estimation

- *Overview of UNIQUE*
- *Unsupervised Learning Mechanism*
- *Preprocessing*
- *Visualization*

## IV. MS-UNIQUE: Multi-model and Sharpness-weighted UNIQUE

- *Multi-model*
- *Sharpness-weighted Multi-model*
- *Visualization*

## V. Validation

## VI. Conclusion

# IV. MS-UNIQUE: Multi-model and Sharpness-weighted UNIQUE

*Multi-model*

Varying the number of neurons to learn global and local features

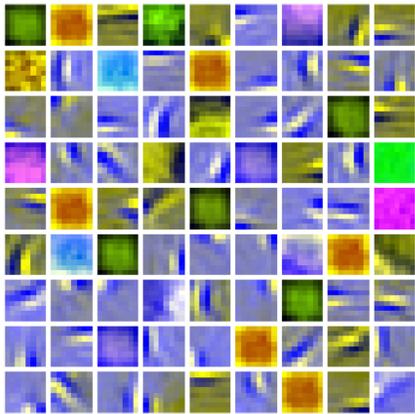

81

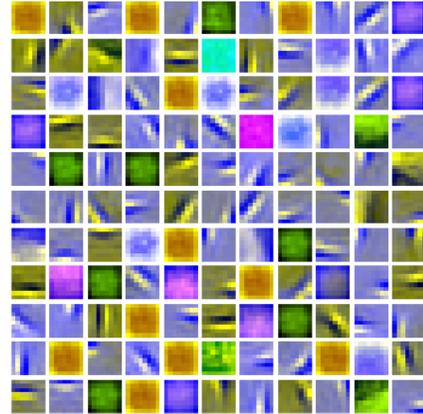

121

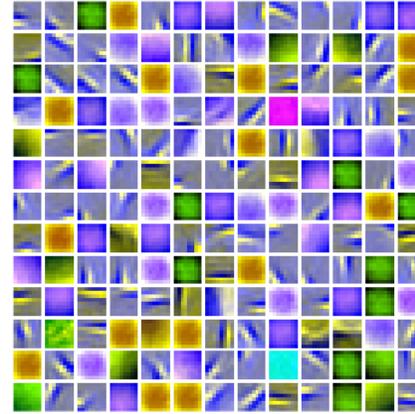

169

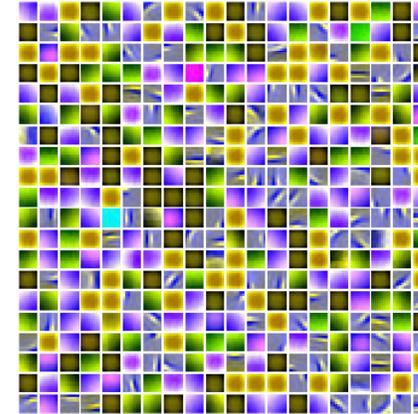

400

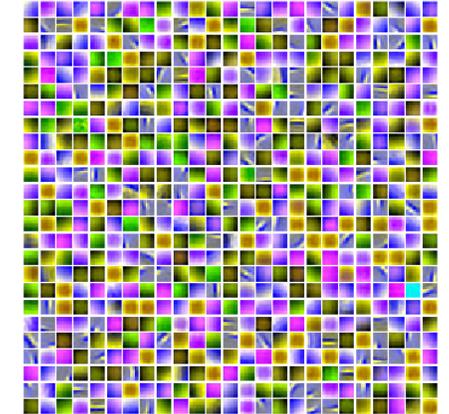

625

# IV. MS-UNIQUE: Multi-model and Sharpness-weighted UNIQUE

*Sharpness-weighted Multi-model*

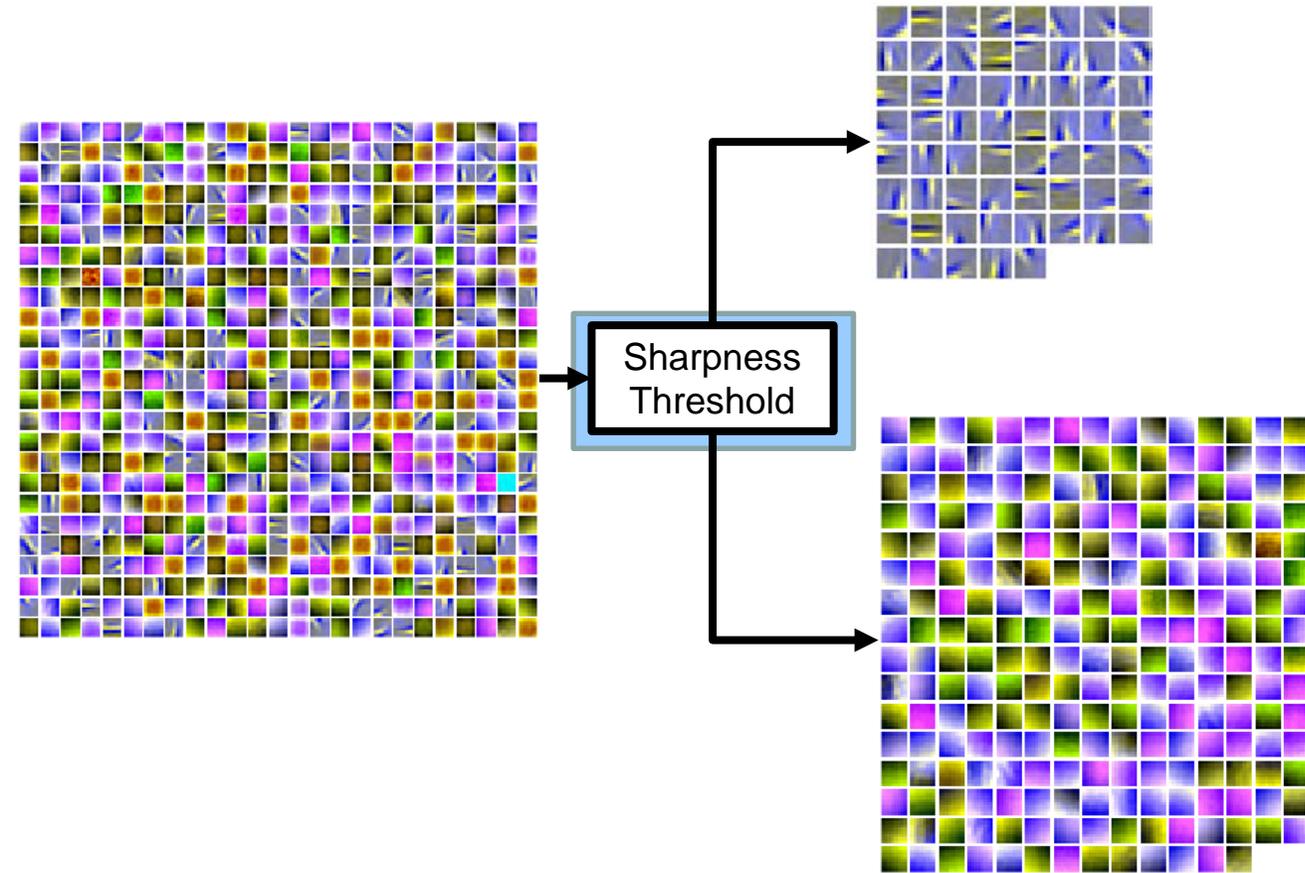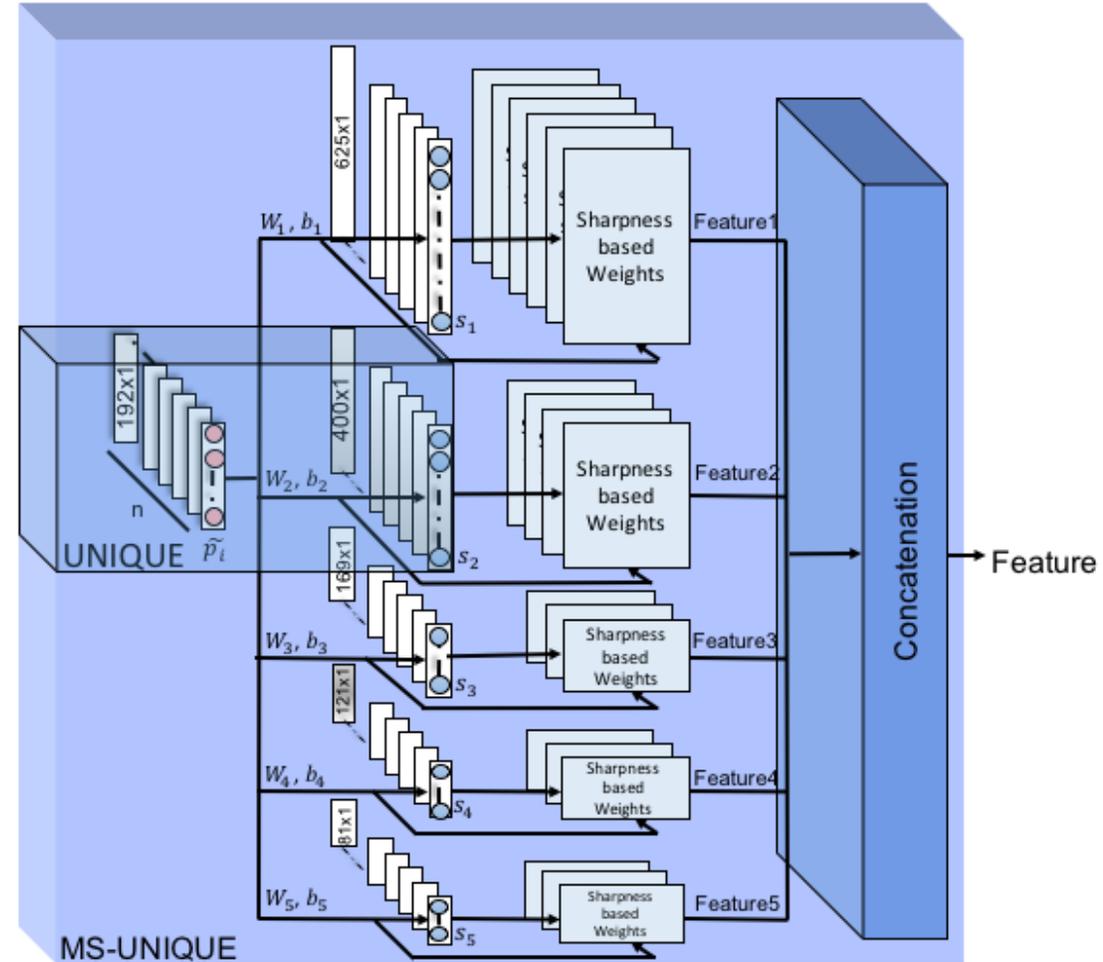

# IV. MS-UNIQUE: Multi-model and Sharpness-weighted UNIQUE

Visualization

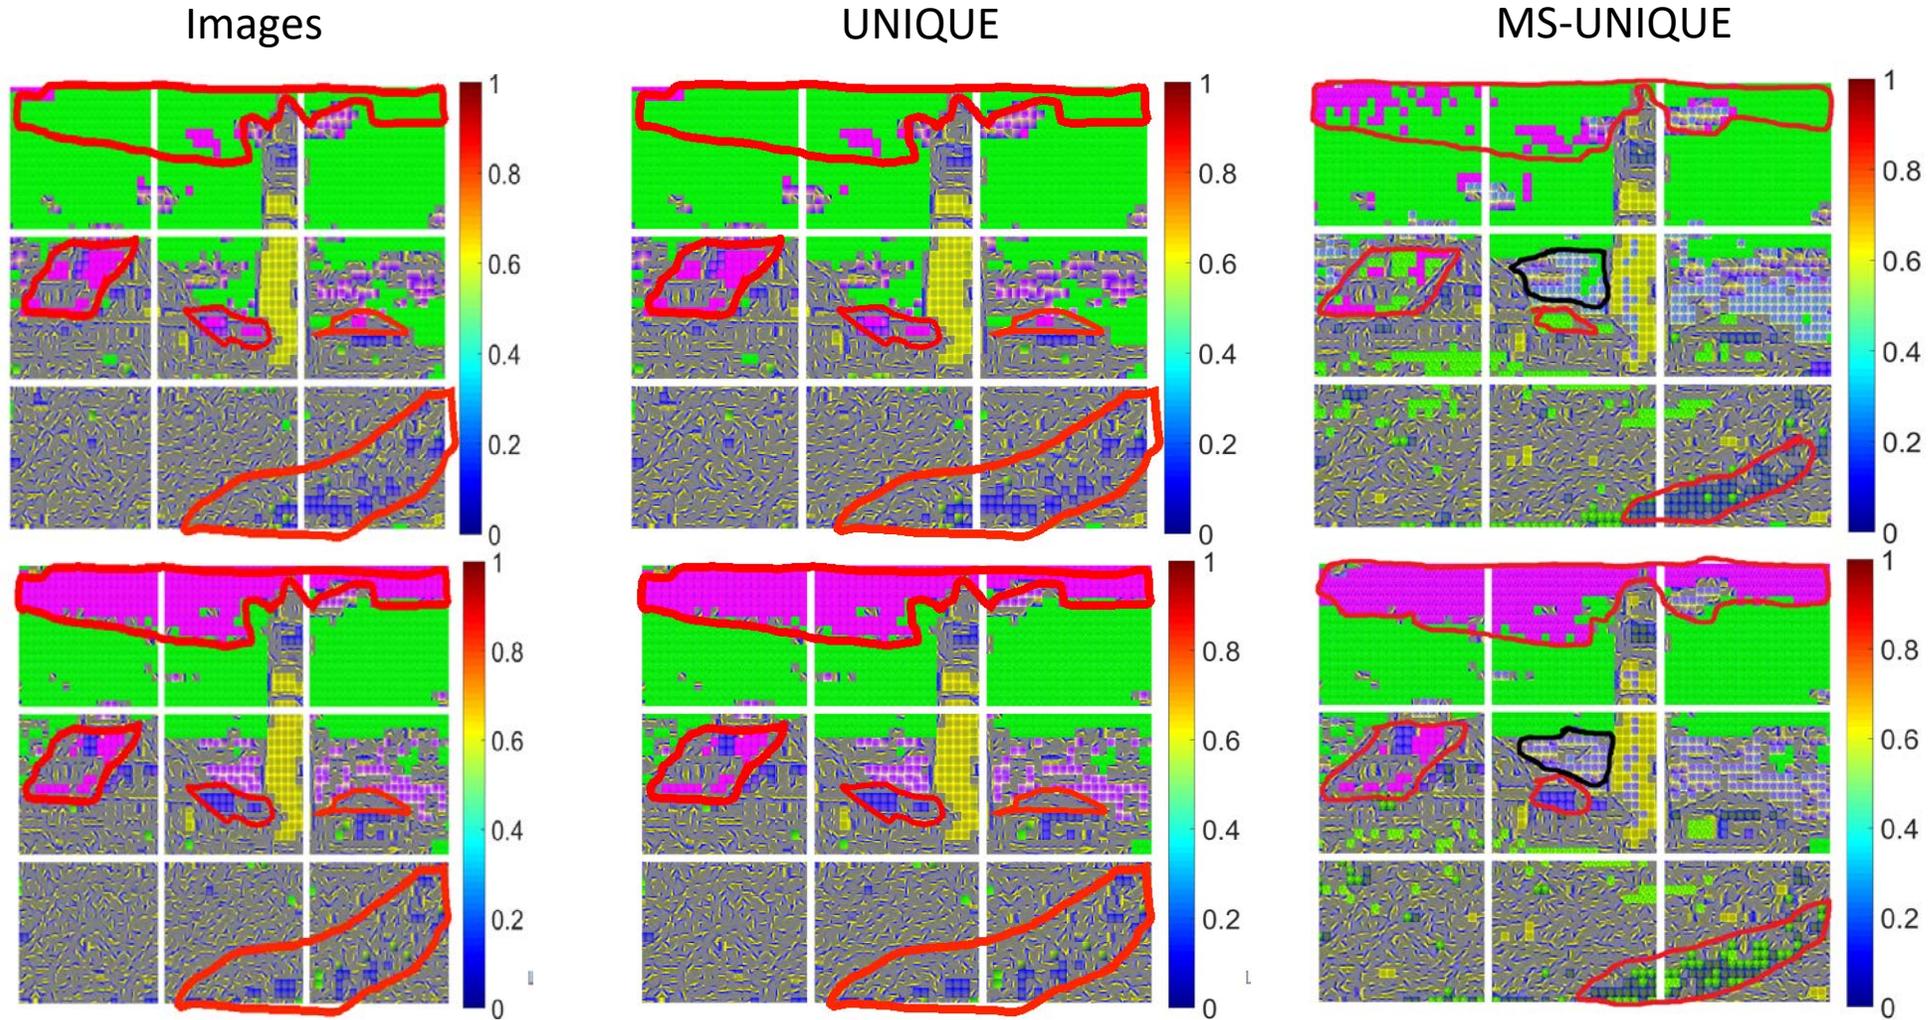

## I. Introduction

## II. Literature Review

## III. UNIQUE: Unsupervised Image Quality Estimation

- *Overview of UNIQUE*
- *Unsupervised Learning Mechanism*
- *Preprocessing*
- *Visualization*

## IV. MS-UNIQUE: Multi-model and Sharpness-weighted UNIQUE

- *Multi-model*
- *Sharpness-weighted Multi-model*
- *Visualization*

## V. Validation

## VI. Conclusion

# V. Image Quality Estimators

- Validation

## Databases

|               | LIVE | TID  | Total |
|---------------|------|------|-------|
| Compression   | 460  | 375  | 835   |
| Image Noise   | 174  | 1375 | 1549  |
| Communication | 174  | 250  | 424   |
| Blur          | 174  | 250  | 424   |
| Color         | -    | 375  | 375   |
| Global        | -    | 250  | 250   |
| Local         | -    | 250  | 250   |

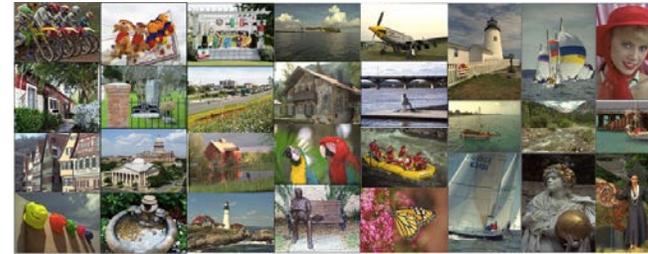

LIVE database

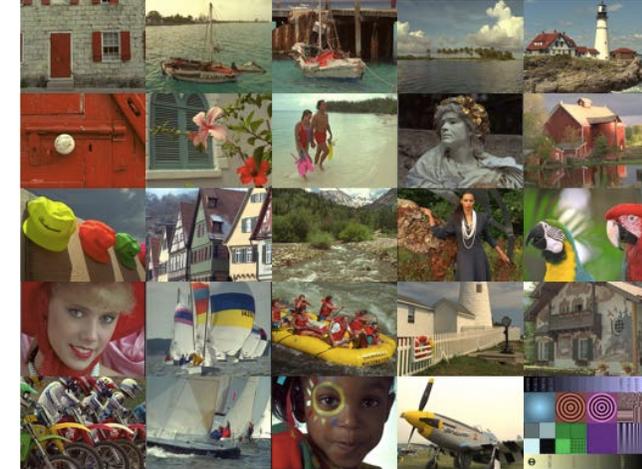

TID 2013 database

## Performance Metrics

| Root mean square error (RMSE)<br><i>Accuracy</i> | Outlier Ratio (OR)<br><i>Consistency</i> | Pearson Linear Correlation Coefficient (PLCC)<br><i>Linearity</i> | Spearman Rank Correlation Coefficient (SRCC)<br><i>Ranking</i>                               |
|--------------------------------------------------|------------------------------------------|-------------------------------------------------------------------|----------------------------------------------------------------------------------------------|
| $\sqrt{E[X - Y]^2}$                              | $\frac{N_{outliers}}{N_{total}}$         | $\frac{E[(X - \mu_X)(Y - \mu_Y)]}{\sigma_X \sigma_Y}$             | $X_i, Y_i \longrightarrow x_i, y_i$<br>$1 - \frac{6 \sum_{i=1}^N (x_i - y_i)^2}{N(N^2 - 1)}$ |

# V. Image Quality Estimators

- Validation

TID13

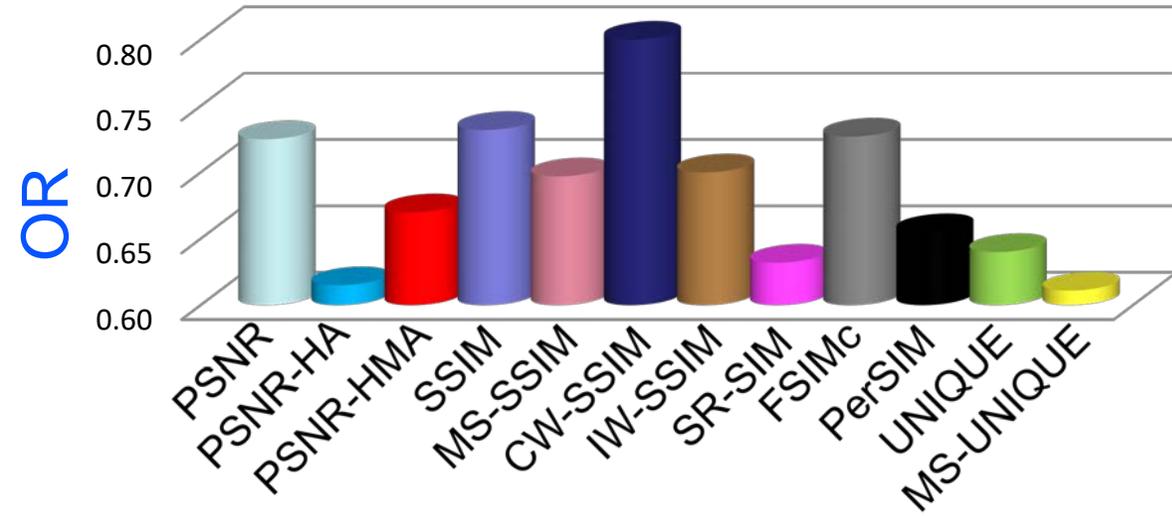

LIVE

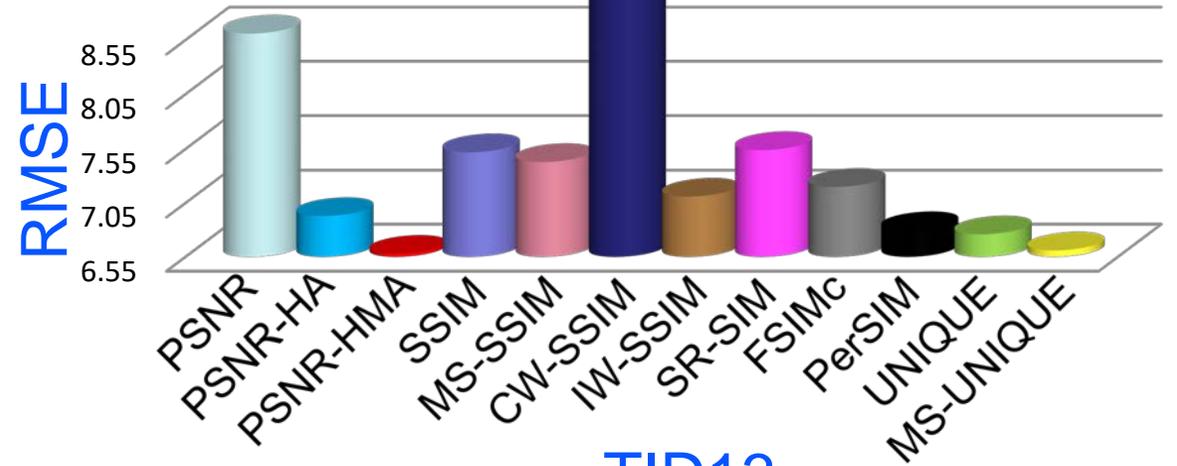

TID13

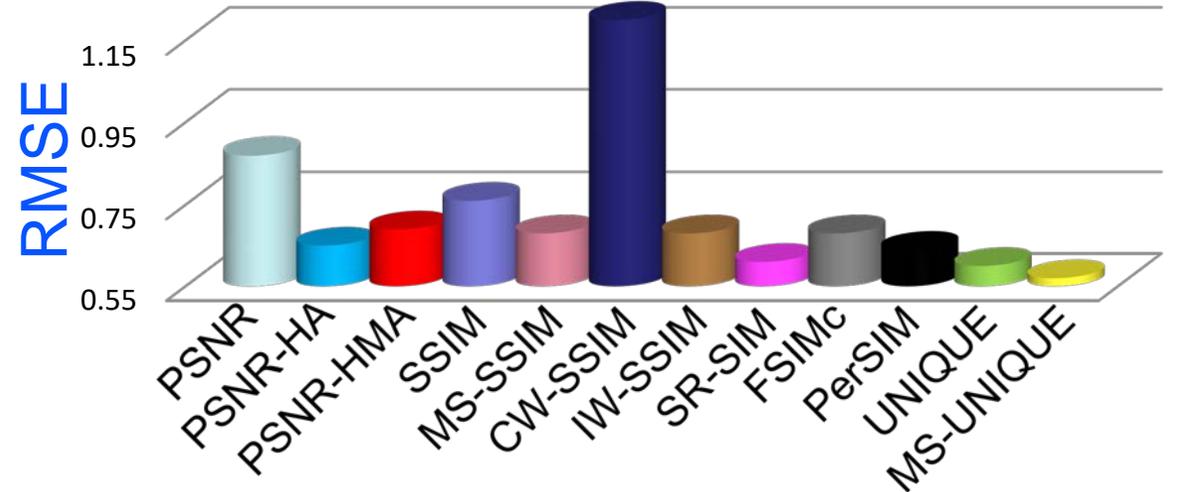

# V. Image Quality Estimators

- Validation

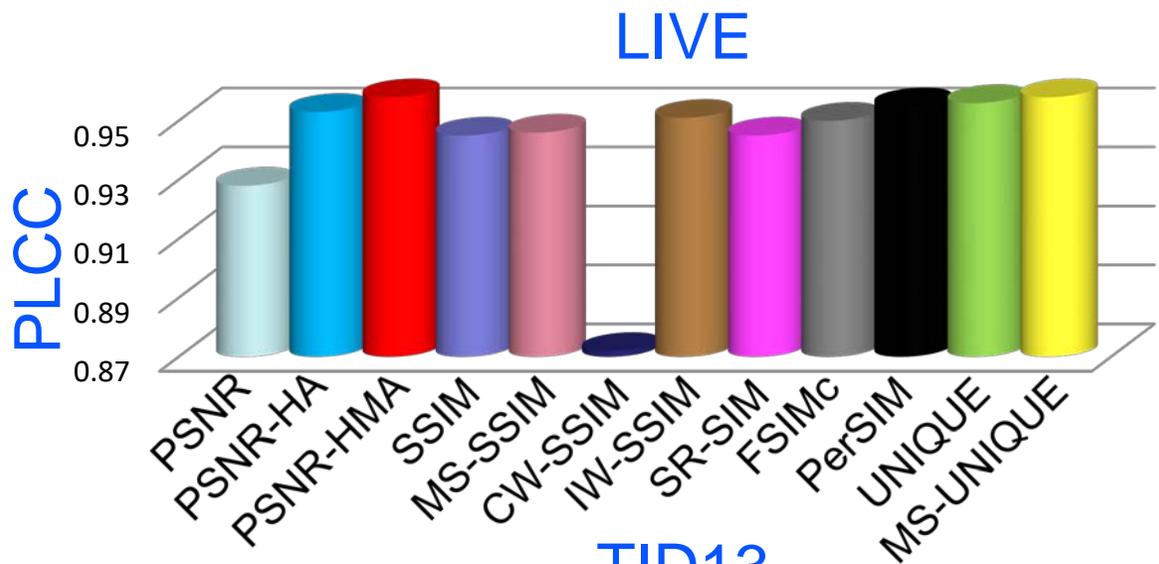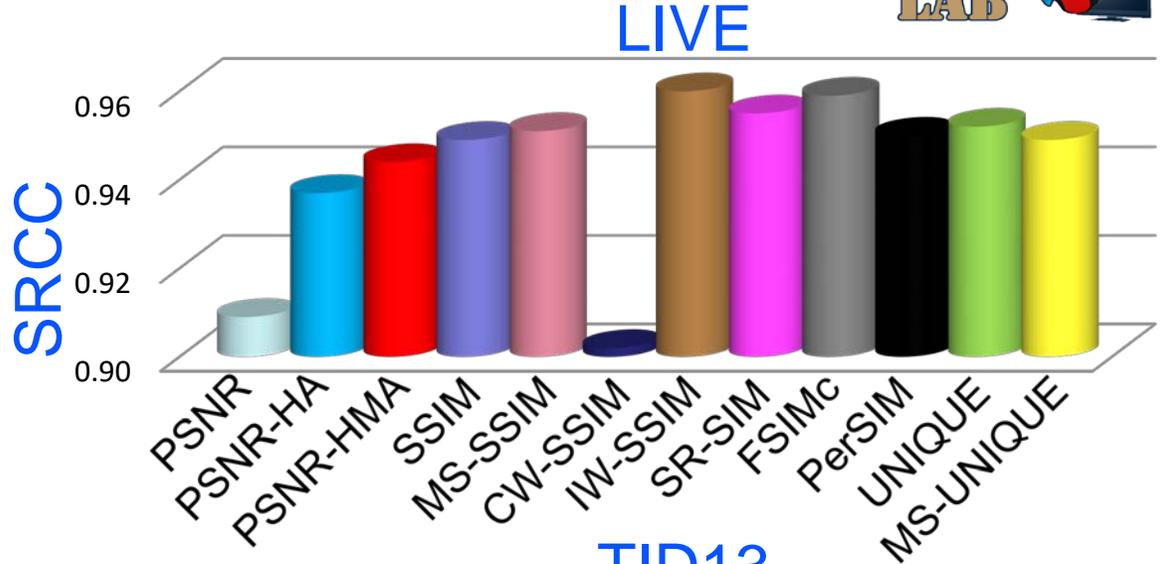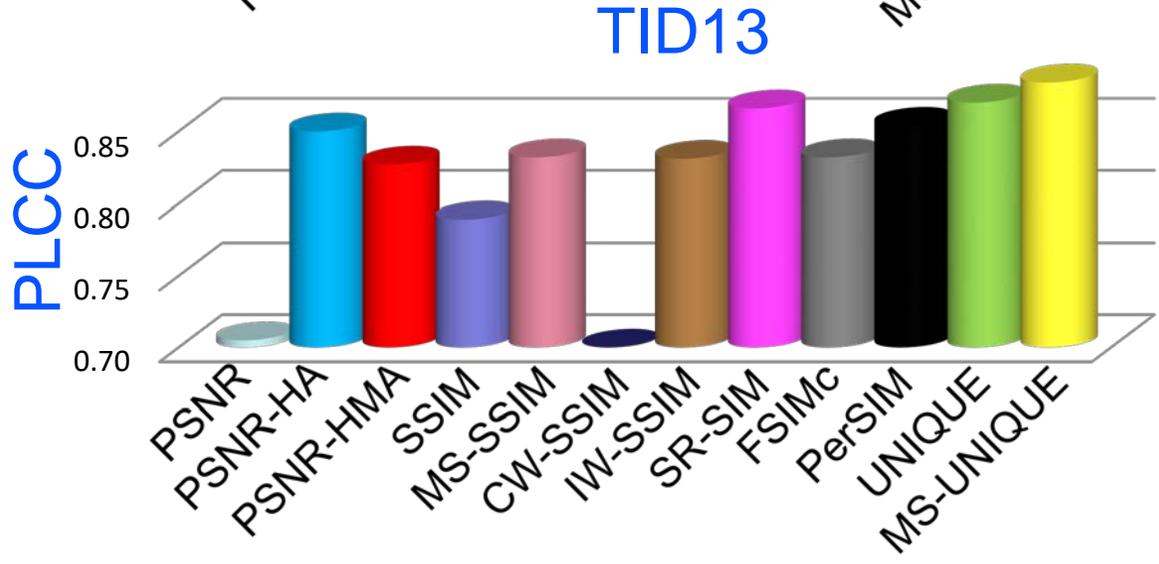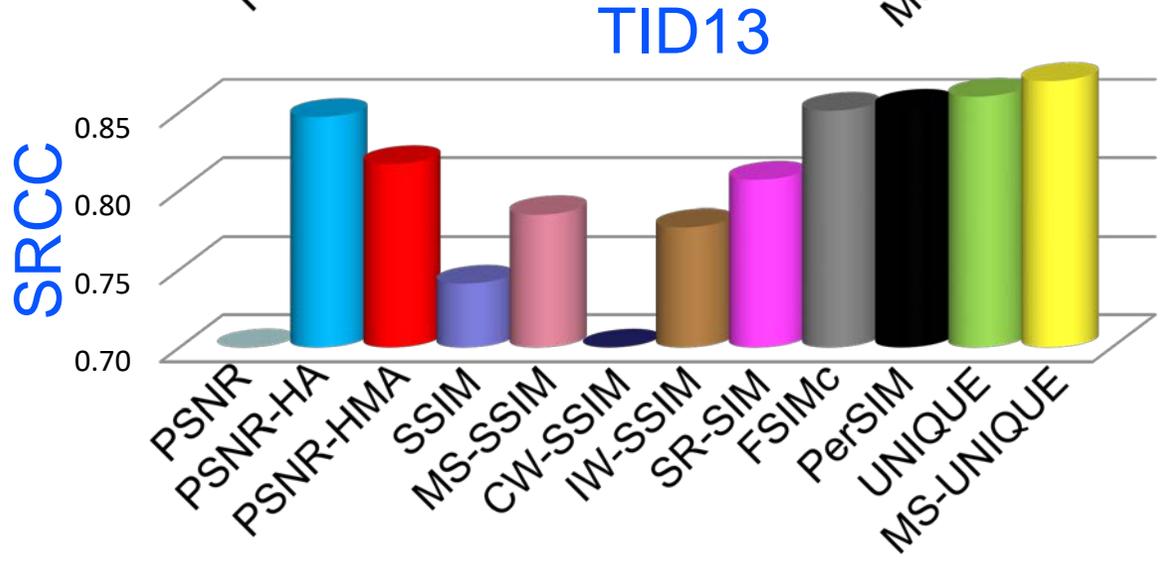

## I. Introduction

## II. Literature Review

## III. UNIQUE: Unsupervised Image Quality Estimation

- *Overview of UNIQUE*
- *Unsupervised Learning Mechanism*
- *Preprocessing*
- *Visualization*

## IV. MS-UNIQUE: Multi-model and Sharpness-weighted UNIQUE

- *Multi-model*
- *Sharpness-weighted Multi-model*
- *Visualization*

## V. Validation

## VI. Conclusion

# VI. Conclusion

## Contributions and Observations

| YEAR                                        |                                          | 2011 |         | 2012   |         |       | 2013  |     |       | 2014 |     |      |       | 2015                  |           |    |                               | 2016  |     |         |        |           |
|---------------------------------------------|------------------------------------------|------|---------|--------|---------|-------|-------|-----|-------|------|-----|------|-------|-----------------------|-----------|----|-------------------------------|-------|-----|---------|--------|-----------|
| QUALITY ESTIMATORS                          |                                          | LBIQ | DIIVINE | CORNIA | BRISQUE | MLIQM | CB/SF | QAC | SPARQ | Tang | QAF | Kang | Qarea | Q <sub>exponent</sub> | IQA-CNN++ | Li | S <sup>2</sup> F <sup>2</sup> | DLIQA | Gao | CNN-SVR | UNIQUE | MS-UNIQUE |
| Visual system                               |                                          |      | ■       |        | ■       | ■     |       | ■   | ■     |      |     |      |       |                       |           | ■  | ■                             | ■     | ■   |         | ■      | ■         |
| Color                                       |                                          |      |         |        | ■       |       |       |     |       |      |     |      |       |                       |           |    |                               |       |     |         | ■      | ■         |
| Do not require                              | Distortion specific data in the training |      |         |        |         |       |       | ■   |       |      |     |      | ■     |                       |           |    |                               |       |     |         | ■      | ■         |
|                                             | Labels in the training                   |      |         |        |         |       | ■     | ■   |       |      |     |      | ■     |                       |           |    |                               |       |     |         | ■      | ■         |
|                                             | Handcrafting                             |      |         | ■      |         |       | ■     |     |       |      |     | ■    |       |                       | ■         |    |                               |       |     | ■       | ■      | ■         |
| Multiple layers/models without handcrafting |                                          |      |         |        |         |       |       |     |       |      |     | ■    |       | ■                     | ■         |    |                               |       |     | ■       |        | ■         |

To measure perceived quality

- Hand-crafting is not sufficient, we should also *learn* from the data.
- Labels are not easy to find, we need to focus more on *unsupervised* approaches.
- *Color perception* must be included in a comprehensive visual system model.
- The best example is our *visual system*, we should model it as much as we can.
